# Supplementary material for: Structure, phonons, and orbital degrees of freedom in Fe$_2$Mo$_3$O$_8$
Source: arXiv:2004.14038 source file (2020-09-25)
Supplement: Supplementary file 1 [file Fe2Mo3O8_Supplement.pdf]

# Supplemental Material

## Structure, phonons, and orbital degrees of freedom in the $\text{Fe}_2\text{Mo}_3\text{O}_8$ multiferroic

S. Reschke,<sup>1</sup> A.A. Tsirlin,<sup>2,\*</sup> N. Khan,<sup>2</sup> V. Tsurkan,<sup>1,3</sup> I. Kézsmárki,<sup>1</sup> and J. Deisenhofer<sup>1,†</sup>

<sup>1</sup>*Experimentalphysik V, Center for Electronic Correlations and Magnetism,  
Institute for Physics, Augsburg University, D-86135 Augsburg, Germany*

<sup>2</sup>*Experimentalphysik VI, Center for Electronic Correlations and Magnetism,  
Institute for Physics, Augsburg University, D-86135 Augsburg, Germany*

<sup>3</sup>*Institute of Applied Physics, MD-2028 Chişinău, Republic of Moldova*

TABLE S1. Phonon frequencies (in  $\text{cm}^{-1}$ ) calculated for crystal structures determined at different temperatures and for two different types of magnetic order, ferromagnetic and antiferromagnetic. The **nonmag** stands for the uncorrelated non-magnetic calculation. All magnetic calculations are performed on the DFT+ $U$ +SO level, where insulating ground state is obtained.

|       | $T = 1.7 \text{ K}$ |  | $T = 1.7 \text{ K}$ |     | $T = 275 \text{ K}$ |     | $T = 1.7 \text{ K}$ |  | $T = 1.7 \text{ K}$ |     | $T = 275 \text{ K}$ |     |
|-------|---------------------|--|---------------------|-----|---------------------|-----|---------------------|--|---------------------|-----|---------------------|-----|
|       | nonmag              |  | FM                  | AFM | FM                  | AFM | nonmag              |  | FM                  | AFM | FM                  | AFM |
| $A_1$ | 724                 |  | 792                 | 787 | 789                 | 784 | 739                 |  | 824                 | 815 | 821                 | 812 |
|       | 694                 |  | 733                 | 734 | 730                 | 730 | 707                 |  | 739                 | 738 | 736                 | 734 |
|       | 547                 |  | 653                 | 651 | 653                 | 651 | 540                 |  | 650                 | 647 | 648                 | 648 |
|       | 461                 |  | 568                 | 558 | 565                 | 563 | 483                 |  | 594                 | 586 | 593                 | 591 |
|       | 423                 |  | 456                 | 454 | 455                 | 452 | 427                 |  | 491                 | 481 | 492                 | 483 |
|       | 387                 |  | 453                 | 444 | 453                 | 447 | 377                 |  | 450                 | 449 | 448                 | 446 |
|       | 275                 |  | 363                 | 365 | 363                 | 365 | 290                 |  | 356                 | 363 | 355                 | 362 |
|       | 236                 |  | 267                 | 262 | 267                 | 264 | 212                 |  | 251                 | 253 | 251                 | 253 |
|       | 154                 |  | 207                 | 201 | 207                 | 203 | 167                 |  | 212                 | 208 | 213                 | 212 |
|       |                     |  |                     |     |                     |     | 132                 |  | 156                 | 155 | 155                 | 154 |
| $A_2$ | 486                 |  | 438                 | 434 | 437                 | 435 | 483                 |  | 431                 | 427 | 428                 | 428 |
|       | 450                 |  | 405                 | 403 | 405                 | 402 | 461                 |  | 416                 | 413 | 417                 | 412 |
|       | 138                 |  | 139                 | 141 | 139                 | 142 | 141                 |  | 141                 | 143 | 141                 | 144 |
| $E_1$ | 691                 |  | 744                 | 750 | 742                 | 745 | 690                 |  | 748                 | 751 | 745                 | 747 |
|       | 558                 |  | 570                 | 577 | 567                 | 570 | 560                 |  | 565                 | 572 | 562                 | 564 |
|       | 522                 |  | 520                 | 522 | 518                 | 520 | 517                 |  | 525                 | 525 | 522                 | 524 |
|       | 490                 |  | 482                 | 481 | 482                 | 480 | 489                 |  | 481                 | 482 | 480                 | 479 |
|       | 449                 |  | 471                 | 473 | 467                 | 467 | 460                 |  | 469                 | 472 | 458                 | 467 |
|       | 437                 |  | 450                 | 455 | 450                 | 448 | 420                 |  | 453                 | 453 | 454                 | 447 |
|       | 307                 |  | 347                 | 351 | 346                 | 351 | 302                 |  | 353                 | 359 | 351                 | 357 |
|       | 295                 |  | 318                 | 312 | 319                 | 313 | 288                 |  | 333                 | 334 | 334                 | 334 |
|       | 221                 |  | 273                 | 286 | 274                 | 282 | 222                 |  | 262                 | 277 | 262                 | 274 |
|       | 195                 |  | 219                 | 223 | 218                 | 222 | 191                 |  | 211                 | 215 | 210                 | 212 |
|       | 163                 |  | 186                 | 191 | 187                 | 189 | 167                 |  | 184                 | 191 | 184                 | 191 |
|       | 146                 |  | 157                 | 162 | 157                 | 159 | 142                 |  | 145                 | 147 | 145                 | 145 |
|       |                     |  |                     |     |                     |     | 44                  |  | 68                  | 77  | 66                  | 71  |

<sup>†</sup> joachim.deisenhofer@physik.uni-augsburg.de  
<sup>\*</sup> altsirlin@gmail.com

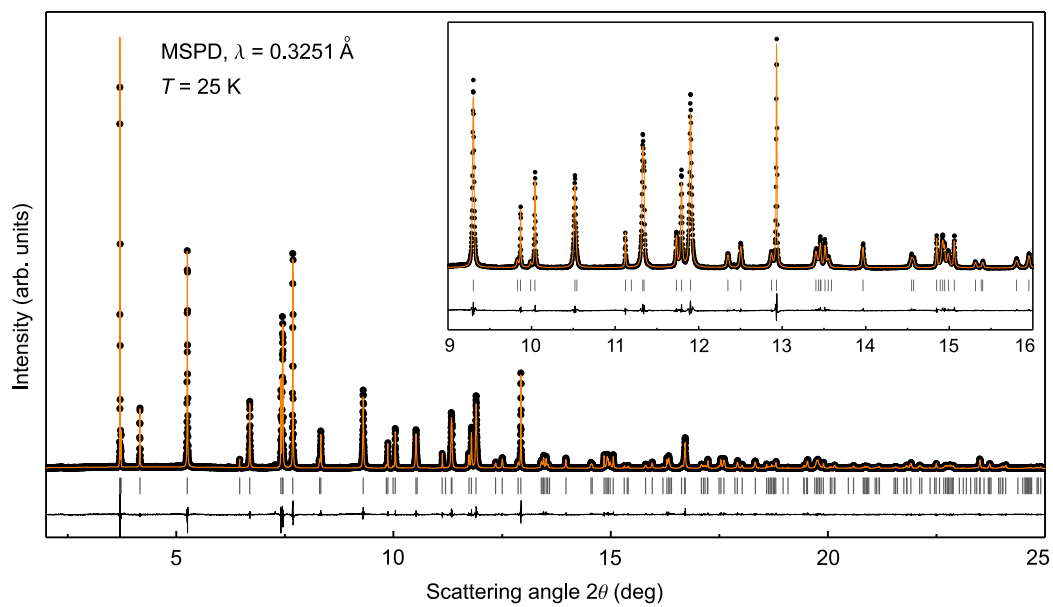

FIG. S1. Rietveld refinement of the synchrotron data collected at 25 K. Tick marks show reflection positions, and the line in the bottom is the difference pattern.
